# Supplementary material for: On the Conditional Existence of Foliations by CMC and Willmore Type Half-Spheres
Source: arXiv:2302.01085 ancillary file (2023-02-02)
Supplement: Supplementary file 1 [file BarycenterCurvePaperCode.pdf]

# Section 4.I - Proof of Equation (4.I7)

We implement the graph function  $u$  from Equation (4.15):

```
In[31]:= u[x_, y_] = a x + a y + x y - c1 x^3 - c2 y^3;
```

## Implementation of the H and Solutions for $c_1$ and $c_2$

To compute the mean curvature of the graph  $(x, y, u(x, y))$  we use the following formula

$$\text{In[6]:= } H = \left[ \left( 1 + (\partial_y u)^2 \right) \partial_{xx} u + \left( 1 + (\partial_x u)^2 \right) \partial_{yy} u - 2 (\partial_y u) (\partial_x u) \partial_{xy} u \right] / \left( \sqrt{1 + (\partial_x u)^2 + (\partial_y u)^2} \right)^3$$

```
In[32]:= H[x_, y_] = ((1 + (D[u[x, y], x])^2) D[u[x, y], {y, 2}] - 2 D[u[x, y], x] D[u[x, y], y]
D[D[u[x, y], x], y] + (1 + (D[u[x, y], y])^2) D[u[x, y], {x, 2}]) /
((1 + (D[u[x, y], x])^2 + (D[u[x, y], y])^2)^(3/2));
```

Next, we implement the gradient of the mean curvature

```
In[33]:= nablH[x_, y_] = {D[H[x, y], x], D[H[x, y], y]};
```

We evaluate at (0,0)

```
In[34]:= nablH0 = FullSimplify[nablH[0, 0]]
```

$$\text{Out[34]= } \left\{ -\frac{2(a - a^3 + 3c_1 + 9a^2c_1 + 6a^4c_1)}{(1 + 2a^2)^{5/2}}, -\frac{2(a - a^3 + 3c_2 + 9a^2c_2 + 6a^4c_2)}{(1 + 2a^2)^{5/2}} \right\}$$

To ensure that (0, 0) is a critical point of H, we set the gradient equal to (0,0) and solve for  $c_1$  and  $c_2$

```
In[35]:= solution = Solve[nablH0 == {0, 0}, {c1, c2}];
```

We save the solutions in new variables newC1 and newC2. Note that the solutions agree with equation (4.16):

```
In[36]:= newC1 = c1 /. solution[[1]]
```

$$\text{Out[36]= } \frac{-a + a^3}{3(1 + 3a^2 + 2a^4)}$$

```
In[37]:= newC2 = c2 /. solution[[1]]
```

$$\text{Out[37]= } \frac{-a + a^3}{3(1 + 3a^2 + 2a^4)}$$

## Implementation of the Gauss curvature

To implement the Gauss curvature, we use the formula

$$K = (\partial_{xx} u \partial_{yy} u - (\partial_{xy} u)^2) / \left( (1 + (\partial_x u)^2 + (\partial_y u)^2)^2 \right)$$

We implement this equation:

```
In[38]:= K[x_, y_] = (D[u[x, y], {x, 2}] D[u[x, y], {y, 2}] - (D[D[u[x, y], x], y])^2) /
  ((1 + (D[u[x, y], x])^2 + (D[u[x, y], y])^2)^2);
```

Next, we define the gradient of the Gauss curvature and evaluate it as (0,0).

```
In[39]:= nablaK[x_, y_] = {D[K[x, y], x], D[K[x, y], y]};
nablaK0 = nablaK[0, 0] /. {c1 -> newC1, c2 -> newC2};;
```

Note that for nabkaK0 we have replaces the parameters c1 and c2 with the parameters newC1 and newC2. Priting nabkaK0 gives the formula claimed in the paper:

```
In[41]:= FullSimplify[nablaK0]
```

```
Out[41]= { 4 a / (1 + 2 a^2)^3, 4 a / (1 + 2 a^2)^3 }
```

## Implemenation of Equation (4.13)

To implement equation (4.13) we first implement the Hessian of H and evaluate at (0,0):

```
In[61]:= HessH[x_, y_] = D[H[x, y], {{x, y}, 2}];
HessH0 = FullSimplify[HessH[0, 0] /. {c1 -> newC1, c2 -> newC2}];
```

Note, that we have also replaced the parameters c1 and c2 with the parameters newC1 and newC2.

We check that this gives the formula provided in the paper:

```
In[63]:= MatrixForm[HessH0]
```

```
Out[63]/MatrixForm=
```

$$\begin{pmatrix} -\frac{2a^2(-5-20a^2+a^4)}{(1+a^2)(1+2a^2)^{7/2}} & -\frac{2(1+4a^2+a^4)}{(1+2a^2)^{7/2}} \\ -\frac{2(1+4a^2+a^4)}{(1+2a^2)^{7/2}} & -\frac{2a^2(-5-20a^2+a^4)}{(1+a^2)(1+2a^2)^{7/2}} \end{pmatrix}$$

The coordinate vector  $\vec{v}_0$  (denoted by vecv0) is given by

```
In[65]:= vecv0 = FullSimplify[Inverse[HessH0].nablaK0]
```

```
Out[65]= { - 2 a (1 + a^2) sqrt(1 + 2 a^2) / (1 - 15 a^4 + 2 a^6), - 2 a (1 + a^2) sqrt(1 + 2 a^2) / (1 - 15 a^4 + 2 a^6) }
```

We compute the euclidean norm of  $\vec{v}_0$  to verify Equation (4.17):

```
In[66]:= Speed[a_] = FullSimplify[Sqrt[FullSimplify[v0.v0]], a >= 0]
```

```
Out[66]= 2 sqrt(2 + 4 a^2) (a + a^3) / Abs[1 - 15 a^4 + 2 a^6]
```

We consider the polynomial in the denominator

```
In[67]:= p[a_] = 1 - 15 a^4 + 2 a^6;
```

We claim that  $p$  has a zero in  $(.5, .52)$ . Indeed

```
In[68]:= p[.5]
```

```
Out[68]= 0.09375
```

```
In[69]:= p[.52]
```

```
Out[69]= -0.0572012
```

# Proof of Equation (5.14) - The linearized CMC Equation

In this Notebook, we construct the solutions for  $g_1$  and  $g_2$  that come up in the process of solving the linearized CMC Equation in Subsection B.3. We then verify that the full solution is indeed a solution to the linearized problem.

## The Solution $g_1$

We have to solve

$$\text{sol1} = \text{DSolve}\left[\frac{1}{\sin[\theta]} D[\sin[\theta] D[g_1[\theta], \theta], \theta] + 2 g_1[\theta] == \frac{3}{2}, g_1[\theta], \theta\right];$$

$$g_1[\theta_] = \text{FullSimplify}[g_1[\theta] /. \text{sol1}[[1]]]$$

$$\frac{3}{4} - C[2] + C[1] \cos[\theta] + \text{ArcTanh}[\cos[\theta]] C[2] \cos[\theta]$$

We know that this function has to satisfy the boundary condition  $\partial_\eta g = -1$ . Note that  $\eta = -\partial_\theta$  and hence we need that  $g_1'(\pi/2) = 1$ . Since

$$D[g_1[\theta], \theta] /. \theta \rightarrow \pi/2 \\ -C[1]$$

we have to take  $C[1] = -1$ . So

$$\text{Betterg}_1[\theta_] = \text{FullSimplify}[g_1[\theta] /. C[1] \rightarrow -1]$$

$$\frac{3}{4} - C[2] - \cos[\theta] + \text{ArcTanh}[\cos[\theta]] C[2] \cos[\theta]$$

The final parameter is eliminated by requiring regularity. To see this, we remark that at  $\theta=0$  we have  $\cos[\theta]=1$  and so  $\text{ArcTanh}[\cos[\theta]]$  is singular at  $\theta=0$ . Indeed we see that for  $C[2]=1$  the function is singular at 0:

$$\text{Plot}[\text{Betterg}_1[\theta] /. C[2] \rightarrow 1, \{\theta, 0, \pi/2\}, \text{PlotRange} \rightarrow \text{All}]$$

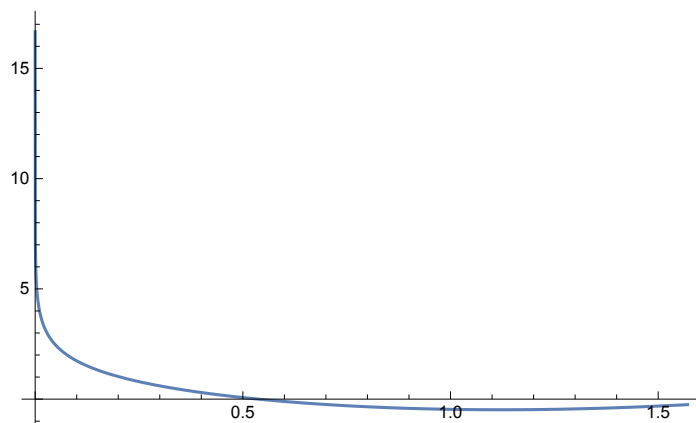

So the correct solution is

$$\text{Finalg}_1[\theta] = \text{Betterg}_1[\theta] /. C[2] \rightarrow 0$$

$$\frac{3}{4} - \cos[\theta]$$

## The Solution $g_2$

We have to solve

$$\text{sol2} = \text{DSolve}[D[G[\theta], \{\theta, 2\}] + 5 \cot[\theta] D[G[\theta], \theta] - 4 G[\theta] == 0, G[\theta], \theta];$$

$$g_2[\theta] = \text{FullSimplify}[G[\theta] /. \text{sol2}[[1]]]$$

$$\frac{\csc[\theta] (C[2] (-3 + \cos[\theta]^2) \cot[\theta] - 3 C[1] \csc[\theta])}{3 \sqrt{-\sin[\theta]^4}}$$

Unfortunately Mathematica gives a Complex solution. We make it real by hand by simply copying this output and replacing  $\text{Sqrt}[-\sin[\theta]^4]$  by  $\sin[\theta]^2$ . The factor of  $i$  is simply absorbed into the constants

$$\text{Modifiedg}_2[\theta] = \frac{\csc[\theta] (C[2] (-3 + \cos[\theta]^2) \cot[\theta] - 3 C[1] \csc[\theta])}{3 \sin[\theta]^2};$$

We know that this function has to satisfy the boundary condition  $\partial_\eta g = -1$ . Note that  $\eta = -\partial_\theta$  and hence we need that  $g_1'(\pi/2) = 1$ . Since

$$BV = D[\text{Modifiedg}_2[\theta], \theta] /. \theta \rightarrow \pi/2$$

$$C[2]$$

we have to take  $C[2]=1$ . So

$$\text{Betterg}_2[\theta] = \text{FullSimplify}[\text{Modifiedg}_2[\theta] /. C[2] \rightarrow 1]$$

$$\frac{1}{12} (-12 C[1] - 9 \cos[\theta] + \cos[3\theta]) \csc[\theta]^4$$

The remaining parameter is eliminated by requiring regularity. We expand around 0:

$$\text{FullSimplify}[\text{Series}[\text{Betterg}_2[\theta], \{\theta, 0, 10\}], 0 \leq \theta \leq \pi/2]$$

$$\begin{aligned} & \frac{-\frac{2}{3} - C[1]}{\theta^4} - \frac{2(2 + 3C[1])}{9\theta^2} + \frac{1}{540}(47 - 132C[1]) + \\ & \frac{(449 - 744C[1])\theta^2}{11340} + \frac{(5147 - 7872C[1])\theta^4}{544320} + \frac{(247 - 372C[1])\theta^6}{133650} + \\ & \frac{(21139367 - 31736832C[1])\theta^8}{65383718400} + \frac{(14009669 - 21018624C[1])\theta^{10}}{267478848000} + O[\theta]^{11} \end{aligned}$$

This shows that  $C[1]=-2/3$

$$\text{Finalg}_2[\theta] = \text{TrigExpand}[\text{Betterg}_2[\theta] /. C[1] \rightarrow -2/3]$$

$$-\frac{1}{4} \cot[\theta] \csc[\theta] + \frac{1}{12} \cot[\theta]^3 \csc[\theta] - \frac{3}{4} \cot[\theta] \csc[\theta]^3 + \frac{2 \csc[\theta]^4}{3}$$

This is not the formula that we claim in the paper and so we check that our formula is indeed the

same. We define

$$\text{Claimedg}_2[\theta] = \frac{1}{3} \frac{(2 - 3 \cos[\theta] + \cos[\theta]^3)}{(1 - \cos[\theta]^2)^2}$$

$$\text{FullSimplify}[\text{Finalg}_2[\theta] - \text{Claimedg}_2[\theta]]$$

$$0$$

## Direct Check

Finally, we can check directly, whether the formula from Equation (5.14) in the paper actually satisfies the linearized problem (B.55). For this we implement the solution

$$\begin{aligned} \omega_1[\theta, \phi] &= \cos[\phi] \sin[\theta]; \\ \omega_2[\theta, \phi] &= \sin[\phi] \sin[\theta]; \\ \omega_3[\theta, \phi] &= \cos[\theta]; \\ f[\theta, \phi] &= (\kappa_1 \omega_1[\theta, \phi]^2 + \kappa_2 \omega_2[\theta, \phi]^2) \omega_3[\theta, \phi]; \\ v_1[\theta, \phi] &= 3/4 - \omega_3[\theta, \phi]; \\ v_2[\theta, \phi] &= (\omega_1[\theta, \phi]^2 - \omega_2[\theta, \phi]^2) / 3 (2 - 3 \omega_3[\theta, \phi] + \omega_3[\theta, \phi]^3) / ((1 - \omega_3[\theta, \phi]^2)^2); \\ v[\theta, \phi] &= 1/4 (\kappa_1 + \kappa_2) v_1[\theta, \phi] + (\kappa_1 - \kappa_2) / 4 v_2[\theta, \phi]; \end{aligned}$$

The graph function derivative  $u'(0)$  is then given by

$$u[\theta, \phi] = v[\theta, \phi] - 1/2 f[\theta, \phi];$$

We also define the correct right hand sides

$$\begin{aligned} \text{PDERHS}[\theta, \phi] &= 5 (\kappa_1 \omega_1[\theta, \phi]^2 + \kappa_2 \omega_2[\theta, \phi]^2) \omega_3[\theta, \phi] - (\kappa_1 + \kappa_2) \omega_3[\theta, \phi] + 3/8 (\kappa_1 + \kappa_2); \\ \text{BCRHS}[\theta, \phi] &= -\kappa_1 \omega_1[\theta, \phi]^2 - \kappa_2 \omega_2[\theta, \phi]^2; \\ \text{IntegralRHS} &= 0; \end{aligned}$$

First we check the PDE

$$\text{FullSimplify}[1/\sin[\theta] D[\sin[\theta] D[u[\theta, \phi], \theta], \theta] + 1/(\sin[\theta]^2) D[u[\theta, \phi], \{\phi, 2\}] + 2 u[\theta, \phi] - \text{PDERHS}[\theta, \phi]]$$

$$0$$

So  $u$  really satisfies the PDE. Next we check the boundary condition

$$\text{FullSimplify}[(-D[u[\theta, \phi], \theta] - \text{BCRHS}[\theta, \phi]) /. \theta \rightarrow \pi/2]$$

$$0$$

So  $u$  satisfies the correct boundary condition. Finally, we need to check the integral condition

$$\text{FullSimplify}[\text{Integrate}[\text{Integrate}[u[\theta, \phi] \sin[\theta], \{\theta, 0, \pi/2\}], \{\phi, 0, 2\pi\}] - \text{IntegralRHS}]$$

$$0$$

# Proof of Equation (5.15)

In this notebook we investigate the second variation of the area functional induced by

$$D_{1,2}^2 A[\theta, \delta] (u'(\theta), g'(\theta)) = \frac{d}{d\epsilon} \frac{d}{d\alpha} A[\epsilon u'(\theta), \delta + \alpha g'(\theta)]$$

For this we first implement the metric and the graph function. First the metric on  $R^3$  from Equation (5.1)

```
q[x_, y_] = {{0, 0, κ1 x}, {0, 0, κ2 y}, {κ1 x, κ2 y, 0}};
G[x_, y_, z_, α_] = IdentityMatrix[3] + α q[x, y];
```

For the graph function from Equation (5.14) we copy code from the graph function notebook:

```
ω1[θ_, φ_] = Cos[φ] Sin[θ];
ω2[θ_, φ_] = Sin[φ] Sin[θ];
ω3[θ_, φ_] = Cos[θ];

f[θ_, φ_] = (κ1 ω1[θ, φ]^2 + κ2 ω2[θ, φ]^2) ω3[θ, φ];
v1[θ_, φ_] = 3/4 - ω3[θ, φ];
v2[θ_, φ_] =
  (ω1[θ, φ]^2 - ω2[θ, φ]^2) / 3 (2 - 3 ω3[θ, φ] + ω3[θ, φ]^3) / ((1 - ω3[θ, φ]^2)^2);
v[θ_, φ_] = 1/4 (κ1 + κ2) v1[θ, φ] + (κ1 - κ2) / 4 v2[θ, φ];
```

The graph function derivative  $u'(0)$ , which we denote by  $u$  in the code, is then given by

```
u[θ_, φ_] = v[θ, φ] - 1/2 f[θ, φ];
```

We now define the parameterization of our surface  $(1+u)\omega$

```
F[θ_, φ_, ε_] = (1 + ε u[θ, φ]) {ω1[θ, φ], ω2[θ, φ], ω3[θ, φ]};
```

We require the metric  $G$  evaluated on the surface

```
GSurface[θ_, φ_, ε_, α_] = FullSimplify[
  G[(1 + ε u[θ, φ]) ω1[θ, φ], (1 + ε u[θ, φ]) ω2[θ, φ], (1 + ε u[θ, φ]) ω3[θ, φ], α];
```

## Expansion of the Gramian

Now we define the first fundamental form

```
g11[θ_, φ_, ε_, α_] = (GSurface[θ, φ, ε, α] . D[F[θ, φ, ε], θ]) . D[F[θ, φ, ε], θ];
g12[θ_, φ_, ε_, α_] = (GSurface[θ, φ, ε, α] . D[F[θ, φ, ε], θ]) . D[F[θ, φ, ε], φ];
g22[θ_, φ_, ε_, α_] = (GSurface[θ, φ, ε, α] . D[F[θ, φ, ε], φ]) . D[F[θ, φ, ε], φ];
```

We implement the Determinant:

```
Detg[θ_, φ_, ε_, α_] = g11[θ, φ, ε, α] g22[θ, φ, ε, α] - g12[θ, φ, ε, α] g12[θ, φ, ε, α];
```

This is a complicated expression of the form

$c_0 + c_1 \epsilon + c_2 \alpha + c_3 \epsilon \alpha + \text{Terms containing } \epsilon^2, \alpha^2$

We only care about the first four terms. So we work the out

```

c0[θ_, φ_] = FullSimplify[Detg[θ, φ, θ, θ]];
c1[θ_, φ_] = FullSimplify[D[Detg[θ, φ, ε, θ], ε] /. ε → 0];
c2[θ_, φ_] = FullSimplify[D[Detg[θ, φ, θ, α], α] /. α → 0];

```

The third coefficient is computationally extensive. So we introduce the following Hilfsfunktion:

```

Hilfsfunktion[θ_, φ_, α_] = D[Detg[θ, φ, ε, α], ε] /. ε → 0;
c3[θ_, φ_] = FullSimplify[D[Hilfsfunktion[θ, φ, α], α] /. α → 0];

```

Lets look at the situation abstractly. We have an expansion of the form

```

Series[Series[Sqrt[a0 + a1 ε + a2 α + a3 ε α], {ε, 0, 1}], {α, 0, 1}]

```

$$\left( \sqrt{a_0} + \frac{a_2 \alpha}{2 \sqrt{a_0}} + O[\alpha]^2 \right) + \left( \frac{a_1}{2 \sqrt{a_0}} + \left( -\frac{a_1 a_2}{4 a_0^{3/2}} + \frac{a_3}{2 \sqrt{a_0}} \right) \alpha + O[\alpha]^2 \right) \epsilon + O[\epsilon]^2$$

Really we only care about the  $\epsilon, \alpha$  term. This we can obtain by computing

```

D[D[Sqrt[a0 + a1 ε + a2 α + a3 ε α], ε], α] /. {ε → 0, α → 0}

```

$$-\frac{a_1 a_2}{4 a_0^{3/2}} + \frac{a_3}{2 \sqrt{a_0}}$$

We define a function in which we replace the a's by the c's

```

j[θ_, φ_] =
FullSimplify[-c1[θ, φ] c2[θ, φ] / (4 Sqrt[c0[θ, φ]]^3) + c3[θ, φ] / (2 Sqrt[c0[θ, φ]])];

```

## Final Computation

We now have that  $d/d\epsilon d/d\alpha A[\epsilon u'(0), \delta + \alpha q] =$

```

Integral = Integrate[Integrate[j[θ, φ], {θ, 0, π/2}], {φ, 0, 2 π}]

```

$$-\frac{\pi (579 \kappa_1^2 + 358 \kappa_1 \kappa_2 + 579 \kappa_2^2)}{2240}$$

Using that  $\kappa_1^2 + \kappa_2^2 = H^2 - 2K$  and  $\kappa_1 \kappa_2 = K$  we can simplify this to the formula we claim in Equation (5.15);

```

Expand[
FullSimplify[Integral /. {κ1 → H/2 + Sqrt[H^2/4 - K], κ2 → H/2 - Sqrt[H^2/4 - K]}]]

```

$$-\frac{579 H^2 \pi}{2240} + \frac{5 K \pi}{14}$$



# Proof of Equations (5.16) and (5.19)

In this notebook we perform all the computations that we require with the first derivative of the graph function  $u'(0)$  from Equation (5.14) in the CMC case.

First we define the function. This we do in several parts

$$\begin{aligned}\omega_1[\theta, \phi] &= \cos[\phi] \sin[\theta]; \\ \omega_2[\theta, \phi] &= \sin[\phi] \sin[\theta]; \\ \omega_3[\theta, \phi] &= \cos[\theta];\end{aligned}$$

Using these, we now define the three parts that make up  $u'(0)$  from Equation (5.14)

$$\begin{aligned}f[\theta, \phi] &= (\kappa_1 \omega_1[\theta, \phi]^2 + \kappa_2 \omega_2[\theta, \phi]^2) \omega_3[\theta, \phi]; \\ v_1[\theta, \phi] &= 3/4 - \omega_3[\theta, \phi]; \\ v_2[\theta, \phi] &= (\omega_1[\theta, \phi]^2 - \omega_2[\theta, \phi]^2) / 3 (2 - 3 \omega_3[\theta, \phi] + \omega_3[\theta, \phi]^3) / ((1 - \omega_3[\theta, \phi]^2)^2); \\ v[\theta, \phi] &= 1/4 (\kappa_1 + \kappa_2) v_1[\theta, \phi] + (\kappa_1 - \kappa_2) / 4 v_2[\theta, \phi];\end{aligned}$$

Finally, we can define the graph function by

$$u[\theta, \phi] = v[\theta, \phi] - 1/2 f[\theta, \phi];$$

## Proof of Equation (5.19) - Computation of $D_1 A[0, \delta] u''(0)$

In Subsection B.5 we prove that  $D_1 A[0, \delta] u''(0) = 2 \int u'' = -4 \int (u')^2 = -4 I_1$ . We first implement  $I_1$ :

$$I_1 = \text{Integrate}[\text{Integrate}[u[\theta, \phi]^2 \sin[\theta], \{\phi, 0, 2\pi\}], \{\theta, 0, \pi/2\}];$$

We multiply by -4 and replace  $\kappa_1$  and  $\kappa_2$  by their respective formulas in terms of  $H$  and  $K$ . This gives Equation (5.19):

$$\begin{aligned}\text{Expand}[\text{FullSimplify}[-4 I_1 /. \{\kappa_1 \rightarrow H/2 + \text{Sqrt}[H^2/4 - K], \kappa_2 \rightarrow H/2 - \text{Sqrt}[H^2/4 - K]\}]] \\ \frac{113 H^2 \pi}{30240} - \frac{229 K \pi}{945} - \frac{1}{9} H^2 \pi \log[2] + \frac{4}{9} K \pi \log[2]\end{aligned}$$

## Proof of Equation (5.16) - Computation of $D_1^2 A[0, \delta](u'(0), u'(0))$

Using the formula for  $u'(0)$  we work out  $d^2/d\epsilon^2 A[\epsilon u'(0), \delta]$ . To do so, we use Equation (B.6) to implement the second variation of the measure

$$\begin{aligned}\text{Measure2}[\theta, \phi] &= \\ (2 u[\theta, \phi]^2 + D[u[\theta, \phi], \theta]^2 + 1 / (\sin[\theta]^2) D[u[\theta, \phi], \phi]^2) \sin[\theta];\end{aligned}$$

We now have to integrate over  $\theta$  and  $\phi$ :

$$\text{I2} = \text{Integrate}[\text{Integrate}[\text{Measure2}[\theta, \phi], \{\theta, 0, \pi/2\}], \{\phi, 0, 2\pi\}]$$

$$\frac{\pi \left( 2201 \kappa_1^2 + 3410 \kappa_1 \kappa_2 + 2201 \kappa_2^2 + 960 (\kappa_1 - \kappa_2)^2 \text{Log}[2] \right)}{8640}$$

Finally we replace  $\kappa_1$  and  $\kappa_2$  by their respective formulas in terms of H and K. This gives Equation (5.16)

$$\text{Expand}[\text{FullSimplify}[\text{I2} /. \{\kappa_1 \rightarrow H/2 + \text{Sqrt}[H^2/4 - K], \kappa_2 \rightarrow H/2 - \text{Sqrt}[H^2/4 - K]\}]]$$

$$\frac{2201 H^2 \pi}{8640} - \frac{31 K \pi}{270} + \frac{1}{9} H^2 \pi \text{Log}[2] - \frac{4}{9} K \pi \text{Log}[2]$$

# Proof of Equation (5.17)

In this document we compute the second variation of the area functional with respect to the linearized metric  $\delta + \epsilon g'(0)$

$$D_2^2 A[0, \delta](g'(0), g'(0)) = \frac{d^2}{d\epsilon^2} A[0, \delta + \epsilon g'(0)]$$

where we use the formula from Equation (5.1)

$$q[x_, y_] = \{\{\theta, \theta, \kappa_1 x\}, \{\theta, \theta, \kappa_2 y\}, \{\kappa_1 x, \kappa_2 y, \theta\}\};$$

$$\text{MatrixForm}[q[x, y]]$$

$$\begin{pmatrix} \theta & \theta & x \kappa_1 \\ \theta & \theta & y \kappa_2 \\ x \kappa_1 & y \kappa_2 & \theta \end{pmatrix}$$

That is, we consider the background metric

$$G[x_, y_, z_, \epsilon_] = \text{IdentityMatrix}[3] + \epsilon q[x, y];$$

We define spherical coordinates

$$f[\theta_, \phi_] = \{\text{Cos}[\phi] \text{Sin}[\theta], \text{Sin}[\phi] \text{Sin}[\theta], \text{Cos}[\theta]\};$$

We implement the metric G evaluated at the spherical coordinates

$$Gsp[\theta_, \phi_, \epsilon_] = G[\text{Cos}[\phi] \text{Sin}[\theta], \text{Sin}[\phi] \text{Sin}[\theta], \text{Cos}[\theta], \epsilon];$$

## First Fundamental Form and Check of Equation (B.37)

Using these, we can define the entries of the first fundamental form:

$$\begin{aligned} g_{11}[\theta_, \phi_, \epsilon_] &= \text{FullSimplify}[(Gsp[\theta, \phi, \epsilon] \cdot D[f[\theta, \phi], \theta]) \cdot D[f[\theta, \phi], \theta]]; \\ g_{12}[\theta_, \phi_, \epsilon_] &= \text{FullSimplify}[(Gsp[\theta, \phi, \epsilon] \cdot D[f[\theta, \phi], \theta]) \cdot D[f[\theta, \phi], \phi]]; \\ g_{22}[\theta_, \phi_, \epsilon_] &= \text{FullSimplify}[(Gsp[\theta, \phi, \epsilon] \cdot D[f[\theta, \phi], \phi]) \cdot D[f[\theta, \phi], \phi]]; \end{aligned}$$

Next, we have to implement the determinant of the first second fundamental form

$$\text{Detg}[\theta_, \phi_, \epsilon_] = \text{FullSimplify}[g_{11}[\theta, \phi, \epsilon] g_{22}[\theta, \phi, \epsilon] - g_{12}[\theta, \phi, \epsilon]^2];$$

This is a polynomial in  $\epsilon$  of degree 2. We extract the coefficients

$$\begin{aligned} c_0[\theta_, \phi_] &= \text{FullSimplify}[\text{Detg}[\theta, \phi, 0]]; \\ c_1[\theta_, \phi_] &= \text{FullSimplify}[D[\text{Detg}[\theta, \phi, \epsilon], \epsilon] /. \epsilon \rightarrow 0]; \\ c_2[\theta_, \phi_] &= \text{FullSimplify}[D[\text{Detg}[\theta, \phi, \epsilon], \{\epsilon, 2\}] /. \epsilon \rightarrow 0] \\ &= -2 (\kappa_1 - \kappa_2)^2 \text{Cos}[\phi]^2 \text{Sin}[\theta]^6 \text{Sin}[\phi]^2 \end{aligned}$$

Really we are of course interested in the expression

$$\text{Series}[\text{Sqrt}[a_0 + a_1 \epsilon + \frac{1}{2} a_2 \epsilon^2], \{\epsilon, 0, 2\}]$$

$$\sqrt{a_0} + \frac{a_1 \epsilon}{2 \sqrt{a_0}} + \frac{(-a_1^2 + 2 a_0 a_2) \epsilon^2}{8 a_0^{3/2}} + O[\epsilon]^3$$

where we have to replace  $a_0$ ,  $a_1$  and  $a_2$  by  $c_0$ ,  $c_1$  and  $c_2$ . The first term gives the standard volume

element. From the second term we can compute the first variation of area:  $d/d\epsilon A[0, G(\epsilon)] =$

$$\text{Integrate}\left[\text{Integrate}\left[\frac{c1[\theta, \phi]}{2 \sqrt{c0[\theta, \phi]}}, \{\theta, 0, \pi/2\}\right], \{\phi, 0, 2\pi\}\right] - \frac{1}{4} \pi (\kappa1 + \kappa2)$$

which we have computed analytically in Equation (B.37) .

## Second Variation of the Area

Now, we can compute the second variation. Note that if we differentiate twice with respect to  $\epsilon$  we get a factor of 2, which we must include

$$\text{Integral} = 2 \text{Integrate}\left[\text{Integrate}\left[\frac{(-c1[\theta, \phi]^2 + 2 c0[\theta, \phi] c2[\theta, \phi])}{8 \sqrt{c0[\theta, \phi]}^3}, \{\theta, 0, \pi/2\}\right], \{\phi, 0, 2\pi\}\right] - \frac{4}{105} \pi (5 \kappa1^2 - 6 \kappa1 \kappa2 + 5 \kappa2^2)$$

Finally we replace the principal curvatures with their formulas in terms of the domains mean curvature  $H$  and its Gauss curvature  $K$ . This gives Equation (5.17)

$$\text{Expand}\left[\text{FullSimplify}\left[\text{Integral} /. \{\kappa1 \rightarrow H/2 + \sqrt{H^2/4 - K}, \kappa2 \rightarrow H/2 - \sqrt{H^2/4 - K}\}\right]\right] - \frac{4 H^2 \pi}{21} + \frac{64 K \pi}{105}$$

# Check of Equation (5.3) - The linearized Willmore Equation

In this notebook we demonstrate that the explicit formula for the graph function does indeed solve the linearized problem. First we implement the solution from Equation (5.3). We follow the Paragraph “Derivation of  $u'(0)$ ” in Subsection B.4. We define

```
 $\omega_1[\theta, \phi] = \cos[\phi] \sin[\theta];$   
 $\omega_2[\theta, \phi] = \sin[\phi] \sin[\theta];$   
 $\omega_3[\theta, \phi] = \cos[\theta];$   
 $f[\theta, \phi] = (\kappa_1 \omega_1[\theta, \phi]^2 + \kappa_2 \omega_2[\theta, \phi]^2) \omega_3[\theta, \phi];$   
 $v_1[\theta, \phi] = 1 - \log[2] + 1/2 \log[1 + \omega_3[\theta, \phi]] - 3/4 \omega_3[\theta, \phi];$   
 $v_2[\theta, \phi] = (\omega_1[\theta, \phi]^2 - \omega_2[\theta, \phi]^2) / (1 + \omega_3[\theta, \phi]);$   
 $v[\theta, \phi] = (\kappa_1 + \kappa_2) v_1[\theta, \phi] + (\kappa_1 - \kappa_2) / 4 v_2[\theta, \phi];$   
 $u[\theta, \phi] = v[\theta, \phi] - 1/2 f[\theta, \phi];$ 
```

In this notebook we write  $u$  instead of  $u'(0)$  since this makes the code more compact. For simplicity we also implement the  $\Delta u$  and  $\Delta^2 u$ . In the spherical coordinate system we have

```
 $\Delta u[\theta, \phi] =$   
 $\text{FullSimplify}[1/\sin[\theta] \mathcal{D}[\sin[\theta] \mathcal{D}[u[\theta, \phi], \theta], \theta] + 1/\sin[\theta]^2 \mathcal{D}[u[\theta, \phi], \{\phi, 2\}]]];$ 
```

Similarly, the Bilaplacian is given by

```
 $\Delta \Delta u[\theta, \phi] =$   
 $\text{FullSimplify}[1/\sin[\theta] \mathcal{D}[\sin[\theta] \mathcal{D}[\Delta u[\theta, \phi], \theta], \theta] + 1/\sin[\theta]^2 \mathcal{D}[\Delta u[\theta, \phi], \{\phi, 2\}]]];$ 
```

---

## PDE Check

We now check that  $u$  is the solution of Equation (B.70). First, we define the left hand side:

```
 $\text{LHS}[\theta, \phi] = \text{FullSimplify}[\Delta \Delta u[\theta, \phi] + 2 \Delta u[\theta, \phi]];$ 
```

To define the right hand side of the PDE we first introduce the following function

```
 $\text{help}[\theta, \phi] = 5 (\kappa_1 \omega_1[\theta, \phi]^2 + \kappa_2 \omega_2[\theta, \phi]^2) \omega_3[\theta, \phi] - (\kappa_1 + \kappa_2) \omega_3[\theta, \phi];$ 
```

The right hand side in the PDE of Equation (B.70) is

```
 $\text{RHS}[\theta, \phi] = \text{FullSimplify}[1/\sin[\theta] \mathcal{D}[\sin[\theta] \mathcal{D}[\text{help}[\theta, \phi], \theta], \theta] +$   
 $1/\sin[\theta]^2 \mathcal{D}[\text{help}[\theta, \phi], \{\phi, 2\}] - (\kappa_1 + \kappa_2)];$ 
```

We now check, whether the right hand side and the left hand side are the same:

```
 $\text{FullSimplify}[\text{LHS}[\theta, \phi] - \text{RHS}[\theta, \phi]]$ 
```

0

## Boundary Condition Check

In Equation (B.70) there are two boundary conditions. We begin with the first order boundary condition. We begin by implementing the left hand side. To do so, we use that  $d/d\eta = -d/d\theta$  at  $\theta = \pi/2$

$$\text{LHSBC1}[\phi] = -D[u[\theta, \phi], \theta] /. \theta \rightarrow \pi/2;$$

Next, we implement the right hand side

$$\text{RHSBC1}[\phi] = -(\kappa_1 \omega_1[\theta, \phi]^2 + \kappa_2 \omega_2[\theta, \phi]^2) /. \theta \rightarrow \pi/2;$$

Now we check, whether the left hand side and the right hand side are equal:

$$\text{FullSimplify}[\text{LHSBC1}[\phi] - \text{RHSBC1}[\phi]]$$

0

Now we repeat the same analysis for the third order boundary condition. First the left hand side

$$\text{LHSBC3}[\phi] = -D[\Delta u[\theta, \phi] + 2u[\theta, \phi], \theta] /. \theta \rightarrow \pi/2;$$

Next, we implement the right hand side

$$\text{RHSBC3}[\phi] = 7(\kappa_1 \omega_1[\theta, \phi]^2 + \kappa_2 \omega_2[\theta, \phi]^2) - (\kappa_1 + \kappa_2) /. \theta \rightarrow \pi/2;$$

Now we check whether the left hand side and the right hand side match up:

$$\text{FullSimplify}[\text{LHSBC3}[\phi] - \text{RHSBC3}[\phi]]$$

0

## Check of the component in the Kernel

The first integral condition, that  $u$  (or  $u'(0)$ ) needs to satisfy is

$$\int u'(\theta) d\mu_{S^2} = \pi / 8 (\kappa_1 + \kappa_2)$$

To check this, we compute the integral on the left hand side:

$$\text{Integrate}[\text{Integrate}[u[\theta, \phi] \text{Sin}[\theta], \{\phi, 0, 2\pi\}], \{\theta, 0, \pi/2\}]$$

$$\frac{1}{8} \pi (\kappa_1 + \kappa_2)$$

The second integral condition is that for  $i=1,2$  the function  $u$  (or  $u'(0)$ ) should satisfy

$$\int u'(\theta) \omega^i d\mu_{S^2} = 0$$

First we check this for  $i=1$ :

$$\text{Integrate}[\text{Integrate}[u[\theta, \phi] \omega_1[\theta, \phi] \text{Sin}[\theta], \{\phi, 0, 2\pi\}], \{\theta, 0, \pi/2\}]$$

0

Next we check the condition for  $i=2$

$$\text{Integrate}[\text{Integrate}[u[\theta, \phi] \omega_2[\theta, \phi] \text{Sin}[\theta], \{\phi, 0, 2\pi\}], \{\theta, 0, \pi/2\}]$$

0

# Proof of Equation (5.4)

In this notebook we verify Equation (5.4). That is we compute

$$D_1^2 \mathcal{W}[0, \delta](u'(0), u'(0))$$

---

## Preliminaries

We define the spherical coordinates

$$\begin{aligned}\omega_1[\theta, \phi] &= \cos[\phi] \sin[\theta]; \\ \omega_2[\theta, \phi] &= \sin[\phi] \sin[\theta]; \\ \omega_3[\theta, \phi] &= \cos[\theta];\end{aligned}$$

Now we implement the linearized graph function  $u'(0)$ , which is denoted by  $u$ , from Equation (5.3):

$$\begin{aligned}f[\theta, \phi] &= (\kappa_1 \omega_1[\theta, \phi]^2 + \kappa_2 \omega_2[\theta, \phi]^2) \omega_3[\theta, \phi]; \\ v_1[\theta, \phi] &= 1 - \log[2] + 1/2 \log[1 + \omega_3[\theta, \phi]] - 3/4 \omega_3[\theta, \phi]; \\ v_2[\theta, \phi] &= (\omega_1[\theta, \phi]^2 - \omega_2[\theta, \phi]^2) / (1 + \omega_3[\theta, \phi]); \\ v[\theta, \phi] &= (\kappa_1 + \kappa_2) v_1[\theta, \phi] + (\kappa_1 - \kappa_2) / 4 v_2[\theta, \phi]; \\ u[\theta, \phi] &= v[\theta, \phi] - 1/2 f[\theta, \phi];\end{aligned}$$

We also implement the Laplacian and the Bilaplacian of  $u$  (or  $u'(0)$ )

$$\begin{aligned}\Delta u[\theta, \phi] &= \\ &\text{FullSimplify}[1/\sin[\theta] D[\sin[\theta] D[u[\theta, \phi], \theta], \theta] + 1/\sin[\theta]^2 D[u[\theta, \phi], \{\phi, 2\}]]; \\ \Delta \Delta u[\theta, \phi] &= \text{FullSimplify}[1/\sin[\theta] D[\sin[\theta] D[\Delta u[\theta, \phi], \theta], \theta] + \\ &\quad 1/\sin[\theta]^2 D[\Delta u[\theta, \phi], \{\phi, 2\}]];\end{aligned}$$

---

## Implementation of the mean curvature

We use the following expansion of the mean curvature, which we establish in Equations (B.13) and (B.14)

$$H[\epsilon u, \delta] = 2 - \epsilon (\Delta + 2) u + 1/2 \epsilon^2 (4 u^2 + 4 u \Delta u) + O(\epsilon^3)$$

Denoting the Taylor coefficients coefficients of the powers of  $\epsilon$  by  $H_0$ ,  $H_1$  and  $H_2$  we

$$\begin{aligned}H_0[\theta, \phi] &= 2; \\ H_1[\theta, \phi] &= -\text{FullSimplify}[2 u[\theta, \phi] + \Delta u[\theta, \phi]]; \\ H_2[\theta, \phi] &= \text{FullSimplify}[4 u[\theta, \phi]^2 + 4 u[\theta, \phi] \Delta u[\theta, \phi]];\end{aligned}$$

This allows us to define the expansion of  $H[\epsilon u, \delta]$  and  $H[\epsilon u, \delta]^2$  up to second order in  $\epsilon$ :

$$\begin{aligned}H[\theta, \phi, \epsilon] &= 2 + \epsilon H_1[\theta, \phi] + 1/2 \epsilon^2 H_2[\theta, \phi]; \\ Hsq[\theta, \phi, \epsilon] &= \text{Series}[H[\theta, \phi, \epsilon]^2, \{\epsilon, 0, 2\}];\end{aligned}$$

---

## Expansion of the Measure

We implement the measure  $d\mu[\epsilon u, \delta]$  up to order  $\epsilon^2$ . To do this we use Equations (B.4) and (B.5).

Also we use that  $d\mu[0,\delta] = \sin[\theta] d\theta d\phi$ :

```
Measure0[θ_, ϕ_] = Sin[θ];
Measure1[θ_, ϕ_] = 2 u[θ, ϕ] Sin[θ];
Measure2[θ_, ϕ_] =
  (2 u[θ, ϕ]^2 + D[u[θ, ϕ], θ]^2 + 1 / (Sin[θ]^2) D[u[θ, ϕ], ϕ]^2) Sin[θ];
```

## Willmore Energy

Using the expansion of  $H^2$  and  $d\mu$  we implemented above, we can implement the Willmore energy

$$\frac{1}{4} \int H[\epsilon u, \delta]^2 d\mu[\epsilon u, \delta]$$

We need to differentiate the integrand twice with respect to  $\epsilon$  and evaluate at  $\epsilon=0$ :

```
Integrand[θ_, ϕ_] =
  D[Series[1/4 Hsq[θ, ϕ, ϵ] Measure[θ, ϕ, ϵ], {ϵ, 0, 2}], {ϵ, 2}] /. ϵ -> 0;
```

We need to integrate over the sphere. As  $W[\theta, \phi]$  already contains the measure, we do not need to include any measure terms:

```
Integral = Integrate[Integrate[Integrand[θ, ϕ], {θ, 0, π/2}], {ϕ, 0, 2π}]
```

$$\frac{1}{280} \pi \left( 863 \kappa_1^2 + 1406 \kappa_1 \kappa_2 + 863 \kappa_2^2 - 840 (\kappa_1 + \kappa_2)^2 \text{Log}[2] \right)$$

Replacing  $a$  and  $b$  by their expressions in terms of  $H$  and  $K$ , we obtain

```
FullSimplify[
  Integral /. {κ1 -> 1/2 (H + Sqrt[H^2 - 4 K]), κ2 -> 1/2 (H - Sqrt[H^2 - 4 K])}]
- 8 K π / 7 + H^2 π (863 / 280 - Log[8])
```



# Proof of Equation (5.5)

In this notebook we compute the derivative

$$D^2_{1,2} \mathcal{W}[\theta, \delta] (u'(\theta), g'(\theta)) = d/d\epsilon d/d\alpha 1/4 \int H[\epsilon u, \delta + \alpha q]^2 d\mu[\epsilon u, \delta + \alpha q]$$

where  $q = g'(0)$

---

## Preliminaries

First we define some useful quantities. The standard basis on  $\mathbb{R}^3$  is given by

$$\begin{aligned} e_1 &= \{1, 0, 0\}; \\ e_2 &= \{0, 1, 0\}; \\ e_3 &= \{0, 0, 1\}; \end{aligned}$$

Next we define spherical coordinates

$$\begin{aligned} \omega_1[\theta, \phi] &= \cos[\phi] \sin[\theta]; \\ \omega_2[\theta, \phi] &= \sin[\phi] \sin[\theta]; \\ \omega_3[\theta, \phi] &= \cos[\theta]; \end{aligned}$$

We collect these in a vector

$$\psi_0[\theta, \phi] = \{\omega_1[\theta, \phi], \omega_2[\theta, \phi], \omega_3[\theta, \phi]\};$$

Next, we implement the metric from Equation (5.1)

$$\begin{aligned} q[x, y] &= \{\{\theta, \phi, \kappa_1 x\}, \{\theta, \phi, \kappa_2 y\}, \{\kappa_1 x, \kappa_2 y, \theta\}\}; \\ \text{tildeg}[x, y, \mu] &= \text{IdentityMatrix}[3] + \alpha q[x, y]; \end{aligned}$$

We define the first derivative of the graph function (that is  $u'(\theta)$ , which we however denote as  $u$  in this notebook) from Equation (5.3)

$$\begin{aligned} f[\theta, \phi] &= (\kappa_1 \omega_1[\theta, \phi]^2 + \kappa_2 \omega_2[\theta, \phi]^2) \omega_3[\theta, \phi]; \\ v_1[\theta, \phi] &= 1 - \log[2] + 1/2 \log[1 + \omega_3[\theta, \phi]] - 3/4 \omega_3[\theta, \phi]; \\ v_2[\theta, \phi] &= (\omega_1[\theta, \phi]^2 - \omega_2[\theta, \phi]^2) / (1 + \omega_3[\theta, \phi]); \\ v[\theta, \phi] &= (\kappa_1 + \kappa_2) v_1[\theta, \phi] + (\kappa_1 - \kappa_2) / 4 v_2[\theta, \phi]; \\ u[\theta, \phi] &= v[\theta, \phi] - 1/2 f[\theta, \phi]; \end{aligned}$$

The surface is parameterized by

$$\psi u[\theta, \phi, \epsilon] = (1 + \epsilon u[\theta, \phi]) \psi_0[\theta, \phi];$$

The metric evaluated on the surface is given by

$$\text{tildegm}[\theta, \phi, \epsilon, \alpha] = \text{tildeg}[\psi u[\theta, \phi, \epsilon].e_1, \psi u[\theta, \phi, \epsilon].e_2, \alpha];$$

---

## First Fundamental Form

We implement the first fundamental form of the surface  $\psi_u$  with respect to the background metric  $\text{tildeg}$

```

g11[θ_, φ_, ε_, α_] = D[ψu[θ, φ, ε], θ].tildegm[θ, φ, ε, α].D[ψu[θ, φ, ε], θ];
g12[θ_, φ_, ε_, α_] = D[ψu[θ, φ, ε], θ].tildegm[θ, φ, ε, α].D[ψu[θ, φ, ε], φ];
g22[θ_, φ_, ε_, α_] = D[ψu[θ, φ, ε], φ].tildegm[θ, φ, ε, α].D[ψu[θ, φ, ε], φ];

```

We collect the entries into a matrix and also introduce the inverse matrix

```

g[θ_, φ_, ε_, α_] =
  {{g11[θ, φ, ε, α], g12[θ, φ, ε, α]}, {g12[θ, φ, ε, α], g22[θ, φ, ε, α]}};
ginv[θ_, φ_, ε_, α_] = Inverse[g[θ, φ, ε, α]];

```

We define the Gramian determinant:

```

Gramm[θ_, φ_, ε_, α_] = Det[g[θ, φ, ε, α]];

```

This function is a series of the form

$$\text{Gramm}[\theta, \phi, \epsilon, \alpha] = \text{Gramm00} + \epsilon \text{Gramm10} + \alpha \text{Gramm01} + \epsilon \alpha \text{Gramm11} + \text{terms with } \epsilon^2 \text{ or } \alpha^2$$

We extract the expansion coefficients. First, we define the first three coefficients

```

Gramm00[θ_, φ_] = FullSimplify[Gramm[θ, φ, 0, 0]];
Gramm10[θ_, φ_] = FullSimplify[D[Gramm[θ, φ, ε, 0], ε] /. ε → 0];
Gramm01[θ_, φ_] = FullSimplify[D[Gramm[θ, φ, 0, α], α] /. α → 0];

```

To define the fourth one, we first define

```

IntermediateGram11[θ_, φ_, ε_] = D[Gramm[θ, φ, ε, α], α] /. α → 0;

```

Using this intermediate function, we compute

```

Gramm11[θ_, φ_] = D[IntermediateGram11[θ, φ, ε], ε] /. ε → 0;

```

We define the integration measure as

```

FullMeasure[θ_, φ_, ε_, α_] =
  Sqrt[Gramm00[θ, φ] + ε Gramm10[θ, φ] + α Gramm01[θ, φ] + ε α Gramm11[θ, φ]];

```

We also define the reduced measure, where we do not include the  $\alpha \epsilon$  term, since this is not necessary for all computations and can thereby reduce the runtime.

```

ReducedMeasure[θ_, φ_, ε_, α_] = Sqrt[Gramm00[θ, φ] + ε Gramm10[θ, φ] + α Gramm01[θ, φ]];

```

## Definition of the Normal

We implement the normal vector, that is presented in Equation (2.4) in the paper. To do this, we first define the following auxilliary quantities:

```

V1[θ_, φ_, ε_, α_] = (tildegm[θ, φ, ε, α].ψ0[θ, φ]).D[ψu[θ, φ, ε], θ];
V2[θ_, φ_, ε_, α_] = (tildegm[θ, φ, ε, α].ψ0[θ, φ]).D[ψu[θ, φ, ε], φ];

```

Equation (2.4) shows that the normal vector points in the following direction

```

N0[θ_, φ_, ε_, α_] = -ψ0[θ, φ] + ginv[θ, φ, ε, α][[1, 1]] V1[θ, φ, ε, α] D[ψu[θ, φ, ε], θ] +
  ginv[θ, φ, ε, α][[1, 2]] V1[θ, φ, ε, α] D[ψu[θ, φ, ε], φ] +
  ginv[θ, φ, ε, α][[2, 1]] V2[θ, φ, ε, α] D[ψu[θ, φ, ε], θ] +
  ginv[θ, φ, ε, α][[2, 2]] V2[θ, φ, ε, α] D[ψu[θ, φ, ε], φ];

```

The norm of this vector squared with respect to the background metric is given by

```

N0Normsq[θ_, φ_, ε_, α_] = (tildegm[θ, φ, ε, α].ψ0[θ, φ]).ψ0[θ, φ] -
  ginv[θ, φ, ε, α][[1, 1]] V1[θ, φ, ε, α] V1[θ, φ, ε, α] -
  ginv[θ, φ, ε, α][[2, 1]] V2[θ, φ, ε, α] V1[θ, φ, ε, α] -
  ginv[θ, φ, ε, α][[1, 2]] V1[θ, φ, ε, α] V2[θ, φ, ε, α] -
  ginv[θ, φ, ε, α][[2, 2]] V2[θ, φ, ε, α] V2[θ, φ, ε, α];

```

We expand N0 and its norm, into a series that includes the terms 1,  $\epsilon$ ,  $\alpha$  and  $\epsilon\alpha$  but no terms containing  $\epsilon^2$  or  $\alpha^2$  since these are not relevant for the current computation

```

BetterN0[θ_, φ_, ε_, α_] = Series[N0[θ, φ, ε, α], {ε, 0, 1}, {α, 0, 1}];
BetterN0Normsq[θ_, φ_, ε_, α_] = Series[N0Normsq[θ, φ, ε, α], {ε, 0, 1}, {α, 0, 1}];

```

Now we can implement the Taylor expansion of the normal vector in Equation (2.4) that includes the terms 1,  $\epsilon$ ,  $\alpha$  and  $\epsilon\alpha$  but no terms containing  $\epsilon^2$  or  $\alpha^2$

```

v[θ_, φ_, ε_, α_] = Series[
  (BetterN0Normsq[θ, φ, ε, α])^(-1/2) BetterN0[θ, φ, ε, α], {ε, 0, 1}, {α, 0, 1}];

```

The relevant coefficients are

```

v00[θ_, φ_] = FullSimplify[v[θ, φ, 0, 0], 0 ≤ θ ≤ π/2];
v10[θ_, φ_] = FullSimplify[D[v[θ, φ, ε, 0], ε] /. ε → 0, 0 ≤ θ ≤ π/2];
v01[θ_, φ_] = FullSimplify[D[v[θ, φ, 0, α], α] /. α → 0, 0 ≤ θ ≤ π/2];
v11[θ_, φ_] = Simplify[D[D[v[θ, φ, ε, α], ε], α] /. {α → 0, ε → 0}];

```

Using these coefficients we can write down the Taylor expansion of the normal as

```

Betterv[θ_, φ_, ε_, α_] = v00[θ, φ] + ε v10[θ, φ] + α v01[θ, φ] + ε α v11[θ, φ];

```

## Second Fundamental Form

To implement the second fundamental form we follow Equation (C.1). First we define the normal parameterization

```

Hilfsψ[θ_, φ_, ε_, α_, z_] = ψu[θ, φ, ε] + z Betterv[θ, φ, ε, α];

```

Now we define the following matrix elements

```

HilfsS11[θ_, φ_, ε_, α_, z_] =
  (tildeg[Hilfsψ[θ, φ, ε, α, z].e1, Hilfsψ[θ, φ, ε, α, z].e2, α].
    D[Hilfsψ[θ, φ, ε, α, z], θ]).D[Hilfsψ[θ, φ, ε, α, z], θ];
HilfsS12[θ_, φ_, ε_, α_, z_] = (tildeg[Hilfsψ[θ, φ, ε, α, z].e1, Hilfsψ[θ, φ, ε, α, z].e2,
  α].D[Hilfsψ[θ, φ, ε, α, z], θ]).D[Hilfsψ[θ, φ, ε, α, z], φ];
HilfsS22[θ_, φ_, ε_, α_, z_] = (tildeg[Hilfsψ[θ, φ, ε, α, z].e1, Hilfsψ[θ, φ, ε, α, z].e2,
  α].D[Hilfsψ[θ, φ, ε, α, z], φ]).D[Hilfsψ[θ, φ, ε, α, z], φ];

```

We collect them into a matrix:

```

HilfsS[θ_, φ_, ε_, α_, z_] = {{HilfsS11[θ, φ, ε, α, z], HilfsS12[θ, φ, ε, α, z]},
  {HilfsS12[θ, φ, ε, α, z], HilfsS22[θ, φ, ε, α, z]}};

```

The matrix HilfsS is the the matrix from Equation (C.2). By Equation (C.1), the second FF is then given by

```

h[θ_, φ_, ε_, α_] = -1/2 D[HilfsS[θ, φ, ε, α, z], z] /. z → 0;

```

This allows us to define the mean curvature as

$$H[\theta_-, \phi_-, \epsilon_-, \alpha_-] = \text{Tr}[\text{ginv}[\theta, \phi, \epsilon, \alpha] \cdot h[\theta, \phi, \epsilon, \alpha]];$$

## Computation of several Terms

Differentiating

$$d / d\epsilon d / d\alpha \int H[\epsilon u, \delta + \alpha q]^2 d\mu[\epsilon u, \delta + \alpha q]$$

using the product rule produces several terms. These are computed separately.

### Term 1

The first term is

$$1/4 \times \int 2 * H[\theta, \delta] d / d\epsilon d / d\alpha H[\epsilon u, \delta + \alpha q] d\mu[\theta, \delta]$$

Using that  $H[0, \delta] = 2$  this simplifies to

$$\int d / d\epsilon d / d\alpha H[\epsilon u, \delta + \alpha q] d\mu[\theta, \delta]$$

So we implement

$$\text{IntegralFunktion1}[\theta_-, \phi_-] = \text{TrigReduce}[D[D[H[\theta, \phi, \epsilon, \alpha], \epsilon], \alpha] /. \{\alpha \rightarrow \theta, \epsilon \rightarrow \theta\}];$$

Since  $d\mu[0, \delta] = \sin[\theta] d\theta d\phi$ , we get

$$\begin{aligned} \text{ResultTerm1} = & \text{Integrate}[\text{Integrate}[\text{IntegralFunktion1}[\theta, \phi] \sin[\theta], \{\theta, 0, \pi/2\}], \{\phi, 0, 2\pi\}] \\ & - \frac{1}{4} (a - b)^2 \pi \end{aligned}$$

### Term 2

The second term is

$$1/4 \int H[\theta, \delta]^2 d / d\epsilon d / d\alpha d\mu[\epsilon u, \delta + \alpha q]$$

which, using  $H[0, \delta] = 2$ , we can simplify to

$$\int d / d\epsilon d / d\alpha d\mu[\epsilon u, \delta + \alpha q]$$

We define

$$\text{IntegralFunktion2}[\theta_-, \phi_-] = D[D[\text{FullMeasure}[\theta, \phi, \epsilon, \alpha], \epsilon] /. \epsilon \rightarrow \theta, \alpha] /. \alpha \rightarrow \theta;$$

Now we integrate

$$\begin{aligned} \text{ResultTerm2} = & \text{Integrate}[\text{Integrate}[\text{IntegralFunktion2}[\theta, \phi], \{\theta, 0, \pi/2\}], \{\phi, 0, 2\pi\}] \\ & \frac{1}{840} \pi \left( -729 a^2 - 1123 a b - 729 b^2 + 630 (a + b)^2 \log[2] \right) \end{aligned}$$

## Term 3

The third term is

$$1/4 \times \int 2 * H[0, \delta] (d / d\epsilon H[\epsilon u, \delta + \alpha q]) d / d\alpha d\mu[\epsilon u, \delta + \alpha q]$$

which, using  $H[0, \delta]=2$ , we can simplify to

$$\int (d / d\epsilon H[\epsilon u, \delta + \alpha q]) d / d\alpha d\mu[\epsilon u, \delta + \alpha q]$$

The integral functions is given by the product of the following two functions. Note that we can use the reduced measure function, since we only take a single derivative of the measure

**IntegralFunktion3Part1** $[\theta_, \phi_] = D[H[\theta, \phi, \epsilon, 0], \epsilon] /. \epsilon \rightarrow 0;$

**IntegralFunktion3Part2** $[\theta_, \phi_] = D[ReducedMeasure[\theta, \phi, 0, \alpha], \alpha] /. \alpha \rightarrow 0;$

The full integration function is then given by the product

**IntegralFunktion3** $[\theta_, \phi_] = \text{IntegralFunktion3Part1}[\theta, \phi] \text{IntegralFunktion3Part2}[\theta, \phi];$

Now we integrate

$$\text{ResultTerm3} = \text{Integrate}[\text{Integrate}[\text{IntegralFunktion3}[\theta, \phi], \{\theta, 0, \pi/2\}], \{\phi, 0, 2\pi\}]$$

$$- \frac{1}{840} \pi \left( -513 a^2 - 776 a b - 513 b^2 + 420 (a + b)^2 \text{Log}[2] \right)$$

## Term 4

The fourth term is

$$1/4 \times \int 2 * H[0, \delta] (d / d\alpha H[0, \delta + \alpha q]) d / d\epsilon d\mu[\epsilon u, \delta]$$

which, using  $H[0, \delta]=2$ , we can simplify to

$$\int (d / d\alpha H[0, \delta + \alpha q]) d / d\epsilon d\mu[\epsilon u, \delta]$$

The integral functions is given by the product of the following two functions. Note that we can use the reduced measure function, since we only take a single derivative of the measure

**IntegralFunktion4Part1** $[\theta_, \phi_] = D[H[\theta, \phi, 0, \alpha], \alpha] /. \alpha \rightarrow 0;$

**IntegralFunktion4Part2** $[\theta_, \phi_] = D[ReducedMeasure[\theta, \phi, \epsilon, 0], \epsilon] /. \epsilon \rightarrow 0;$

The full integration function is then given by the product

**IntegralFunktion4** $[\theta_, \phi_] = \text{IntegralFunktion4Part1}[\theta, \phi] \text{IntegralFunktion4Part2}[\theta, \phi];$

Now we integrate

$$\text{ResultTerm4} = \text{Integrate}[\text{Integrate}[\text{IntegralFunktion4}[\theta, \phi], \{\theta, 0, \pi/2\}], \{\phi, 0, 2\pi\}]$$

$$\frac{1}{420} \pi \left( 216 a^2 + 347 a b + 216 b^2 - 210 (a + b)^2 \text{Log}[2] \right)$$

## Term 5

The fifth term is

$$1/4 \times \int 2 * (d / d\epsilon H[\epsilon u, \delta]) (d / d\alpha H[\theta, \delta + \alpha q]) d\mu[\theta, \delta]$$

which we can simplify to

$$1/2 \int (d / d\epsilon H[\epsilon u, \delta]) (d / d\alpha H[\theta, \delta + \alpha q]) d\mu[\theta, \delta]$$

The integral functions is given by the product of the following two functions

`IntegralFunktion5Part1[θ_, φ_] = D[H[θ, φ, θ, α], α] /. α → θ;`

`IntegralFunktion5Part2[θ_, φ_] = D[H[θ, φ, ε, θ], ε] /. ε → θ;`

The full integration function is then given by the product

`IntegralFunktion5[θ_, φ_] = Simplify[  
  IntegralFunktion5Part1[θ, φ] IntegralFunktion5Part2[θ, φ], TimeConstraint → 1];`

Now we integrate over  $\phi$  and include the factor  $1/2$  that is in front of the integral

`ResultTerm5Step1[θ_] = 1/2 Integrate[IntegralFunktion5[θ, φ], {φ, 0, 2 π}];`

Finally we integrate over  $\theta$  and include factor  $\sin[\theta]$  from the measure  $d\mu[0, \delta]$ .

`ResultTerm5 = Integrate[ResultTerm5Step1[θ] Sin[θ], {θ, 0, π/2}]`

$$\frac{1}{336} \pi \left( -177 a^2 - 104 a b - 177 b^2 + 84 (a + b)^2 \log[2] \right)$$

## Combination of all Terms

The full result is given by

`FullResult =`

`FullSimplify[ResultTerm1 + ResultTerm2 + ResultTerm3 + ResultTerm4 + ResultTerm5]`

$$-\frac{1}{560} (291 a^2 - 338 a b + 291 b^2) \pi$$

Now we replace  $a$  and  $b$  by the formulas in terms of  $H$  and  $K$ . This gives Equation (5.5)

`Expand[FullResult /. {a → 1/2 (H + Sqrt[H^2 - 4 K]), b → 1/2 (H - Sqrt[H^2 - 4 K])}]`

$$-\frac{291 H^2 \pi}{560} + \frac{23 K \pi}{14}$$

# Proof of Equation (5.6)

In this notebook, we compute the following variation:

$$D_2^2 \mathcal{W}[\theta, \delta] (g'(\theta), g'(\theta)) = 1/4 \, d^2 / d\epsilon^2 \int (H[\theta, \delta + \epsilon q])^2 d\mu[\theta, \delta + \epsilon q]$$

where  $q=g'(\theta)$

---

## Preliminaries

The first thing we introduce is the standard basis on  $R^3$ :

```
Subscript[e, 1] = {1, 0, 0};  
e1 = {1, 0, 0};  
Subscript[e, 2] = {0, 1, 0};  
e2 = {0, 1, 0};  
Subscript[e, 3] = {0, 0, 1};  
e3 = {0, 0, 1};
```

Next we define the background metric on  $R^3$ . By Equation (5.1)

```
q[x_, y_] = {{0, 0, x1 x}, {0, 0, x2 y}, {x1 x, x2 y, 0}};  
tildeg[x_, y_, ε_] = IdentityMatrix[3] + ε q[x, y];
```

Next we implement spherical coordinates. These parameterize the sphere

```
ψ[θ_, φ_] = {Sin[θ] Cos[φ], Sin[θ] Sin[φ], Cos[θ]};
```

We also introduce the metric evaluated along the surface

```
tildegψ[θ_, φ_, ε_] = tildeg[ψ[θ, φ][[1]], ψ[θ, φ][[2]], ε];
```

---

## The first Fundamental Form

Using  $\psi$  and the definition of the background metric, we define the first fundamental form of the half sphere with respect to the background metric  $\tilde{\text{deg}}$

```
g11[θ_, φ_, ε_] = (tildeg[ψ[θ, φ].e1, ψ[θ, φ].e2, ε].D[ψ[θ, φ], θ]).D[ψ[θ, φ], θ];  
g12[θ_, φ_, ε_] = (tildeg[ψ[θ, φ].e1, ψ[θ, φ].e2, ε].D[ψ[θ, φ], θ]).D[ψ[θ, φ], φ];  
g22[θ_, φ_, ε_] = (tildeg[ψ[θ, φ].e1, ψ[θ, φ].e2, ε].D[ψ[θ, φ], φ]).D[ψ[θ, φ], φ];
```

We collect the entries into a matrix

```
gm[θ_, φ_, ε_] = {{g11[θ, φ, ε], g12[θ, φ, ε]}, {g12[θ, φ, ε], g22[θ, φ, ε]}};
```

For later use we also introduce the inverse

```
gminv[θ_, φ_, ε_] = Inverse[gm[θ, φ, ε]];
```

---

## Definition of the Normal

We implement the normal vector, that is presented in Equation (2.4) in the paper. To do this, we first define the following auxilliary qunatities:

$$\begin{aligned} V1[\theta_-, \phi_-, \epsilon_-] &= (\text{tildeg}\psi[\theta, \phi, \epsilon] \cdot \psi[\theta, \phi]) \cdot D[\psi[\theta, \phi], \theta]; \\ V2[\theta_-, \phi_-, \epsilon_-] &= (\text{tildeg}\psi[\theta, \phi, \epsilon] \cdot \psi[\theta, \phi]) \cdot D[\psi[\theta, \phi], \phi]; \end{aligned}$$

Equation (2.4) shows that the normal vector points in the following direction

$$\begin{aligned} N0[\theta_-, \phi_-, \epsilon_-] &= -\psi[\theta, \phi] + gminv[\theta, \phi, \epsilon] [[1, 1]] V1[\theta, \phi, \epsilon] D[\psi[\theta, \phi], \theta] + \\ &\quad gminv[\theta, \phi, \epsilon] [[1, 2]] V1[\theta, \phi, \epsilon] D[\psi[\theta, \phi], \phi] + gminv[\theta, \phi, \epsilon] [[2, 1]] \\ &\quad V2[\theta, \phi, \epsilon] D[\psi[\theta, \phi], \theta] + gminv[\theta, \phi, \epsilon] [[2, 2]] V2[\theta, \phi, \epsilon] D[\psi[\theta, \phi], \phi]; \end{aligned}$$

The norm of this vector squared with respect to the background metric is given by

$$\begin{aligned} N0Normsq[\theta_-, \phi_-, \epsilon_-] &= \\ &(\text{tildeg}\psi[\theta, \phi, \epsilon] \cdot \psi[\theta, \phi]) \cdot \psi[\theta, \phi] - gminv[\theta, \phi, \epsilon] [[1, 1]] V1[\theta, \phi, \epsilon] V1[\theta, \phi, \epsilon] - \\ &\quad gminv[\theta, \phi, \epsilon] [[2, 1]] V2[\theta, \phi, \epsilon] V1[\theta, \phi, \epsilon] - gminv[\theta, \phi, \epsilon] [[1, 2]] \\ &\quad V1[\theta, \phi, \epsilon] V2[\theta, \phi, \epsilon] - gminv[\theta, \phi, \epsilon] [[2, 2]] V2[\theta, \phi, \epsilon] V2[\theta, \phi, \epsilon]; \end{aligned}$$

We expand N0 and its norm, into a series that includes the terms up to  $\epsilon^2$ . The higher order terms are not relevant for the current computation

$$\begin{aligned} \text{BetterN0}[\theta_-, \phi_-, \epsilon_-] &= \text{Series}[N0[\theta, \phi, \epsilon], \{\epsilon, 0, 2\}]; \\ \text{BetterN0Normsq}[\theta_-, \phi_-, \epsilon_-] &= \text{Series}[N0Normsq[\theta, \phi, \epsilon], \{\epsilon, 0, 2\}]; \end{aligned}$$

Now we can implement the Taylor expansion of the normal vector in Equation (2.4) that includes terms up to  $\epsilon^2$

$$v[\theta_-, \phi_-, \epsilon_-] = \text{Series}[(\text{BetterN0Normsq}[\theta, \phi, \epsilon])^{(-1/2)} \text{BetterN0}[\theta, \phi, \epsilon], \{\epsilon, 0, 2\}];$$

The relevant coefficients are

$$\begin{aligned} v0[\theta_-, \phi_-] &= \text{FullSimplify}[v[\theta, \phi, 0], 0 \leq \theta \leq \pi/2]; \\ v1[\theta_-, \phi_-] &= \text{FullSimplify}[D[v[\theta, \phi, \epsilon], \epsilon] /. \epsilon \rightarrow 0, 0 \leq \theta \leq \pi/2]; \\ v2[\theta_-, \phi_-] &= \text{Simplify}[D[v[\theta, \phi, \epsilon], \{\epsilon, 2\}] /. \{\epsilon \rightarrow 0\}]; \end{aligned}$$

Using these coefficients we can write down the Taylor expansion of the normal as

$$\text{Betterv}[\theta_-, \phi_-, \epsilon_-] = v0[\theta, \phi] + \epsilon v1[\theta, \phi] + 1/2 \epsilon^2 v2[\theta, \phi];$$

## Computation of the second Fundamental Form

We sue EQuation (C.1) to implement the second fundamental form. First we define the normal parameterization

$$p[\theta_-, \phi_-, \epsilon_-, z_-] = \psi[\theta, \phi] + z \text{Betterv}[\theta, \phi, \epsilon];$$

Now we define an auxiliary matrix

$$\begin{aligned} s11[\theta_-, \phi_-, \epsilon_-, z_-] &= \\ &(\text{tildeg}[p[\theta, \phi, \epsilon, z] \cdot e1, p[\theta, \phi, \epsilon, z] \cdot e2, \epsilon] \cdot D[p[\theta, \phi, \epsilon, z], \theta]) \cdot \\ &\quad D[p[\theta, \phi, \epsilon, z], \theta]; \\ s12[\theta_-, \phi_-, \epsilon_-, z_-] &= (\text{tildeg}[p[\theta, \phi, \epsilon, z] \cdot e1, p[\theta, \phi, \epsilon, z] \cdot e2, \epsilon] \cdot \\ &\quad D[p[\theta, \phi, \epsilon, z], \theta]) \cdot D[p[\theta, \phi, \epsilon, z], \phi]; \\ s22[\theta_-, \phi_-, \epsilon_-, z_-] &= (\text{tildeg}[p[\theta, \phi, \epsilon, z] \cdot e1, p[\theta, \phi, \epsilon, z] \cdot e2, \epsilon] \cdot \\ &\quad D[p[\theta, \phi, \epsilon, z], \phi]) \cdot D[p[\theta, \phi, \epsilon, z], \phi]; \end{aligned}$$

We collect these entries into the matrix from Equation (C.2):



```
s[θ_, φ_, ε_, z_] =
  {{s11[θ, φ, ε, z], s12[θ, φ, ε, z]}, {s12[θ, φ, ε, z], s22[θ, φ, ε, z]}};
```

We obtain the second fundamental form as

```
h[θ_, φ_, ε_] = -1 / D[s[θ, φ, ε, z], z] /. z -> 0;
```

To access the mean curvature we multiply with the inverse of the first FF and take the trace:

```
H[θ_, φ_, ε_] = Tr[gminv[θ, φ, ε] . h[θ, φ, ε]];
```

## Variation of the Measure

We introduce the Grammian Determinant

```
GrammDet[θ_, φ_, ε_] = Det[gm[θ, φ, ε]];
```

As this is a complicated function we access its Taylor Coefficients

```
Ableitung0[θ_, φ_] = FullSimplify[GrammDet[θ, φ, 0]];
Ableitung1[θ_, φ_] = FullSimplify[D[GrammDet[θ, φ, ε], ε] /. ε -> 0];
Ableitung2[θ_, φ_] = FullSimplify[D[D[GrammDet[θ, φ, ε], ε], ε] /. ε -> 0];
```

Using these, we can expand the measure up to  $\epsilon^2$ . To do this, we consider the following 'Hilfsfunktion'

```
Hilfsfunktion[A_, B_, C_, ε_] = Series[Sqrt[A + B ε + 1/2 C ε^2], {ε, 0, 2}]
```

$$\sqrt{A} + \frac{B \epsilon}{2 \sqrt{A}} + \frac{(-B^2 + 2 A C) \epsilon^2}{8 A^{3/2}} + O[\epsilon]^3$$

In this formula A, B and C are placeholders for Ableitung0, Ableitung1 and Ableitung 2 respectively. Let us extract the  $\epsilon^2$  coefficient

## The first Term

We begin by computing the following term:

$$1/4 \int d\theta^2 / d\epsilon^2 (H[\theta, \delta + \epsilon q])^2 d\mu[\theta, \delta]$$

To do this, we need to take the second derivative of  $H[0, \delta + \epsilon q]^2$  with respect to  $\epsilon$  at  $\epsilon=0$

```
Intfunc[θ_, φ_] = D[H[θ, φ, ε]^2, {ε, 2}] /. ε -> 0;
```

We simplify the resulting function to speed up the integration

```
betterIntfunc[θ_, φ_] = FullSimplify[Intfunc[θ, φ]];
```

Finally we can integrate this function. We must include the measure  $d\mu[0, \delta] = \sin[\theta] d\theta d\phi$ . This gives

```
Ergebnis1 =
  1/4 Integrate[Integrate[betterIntfunc[θ, φ] Sin[θ], {φ, 0, 2 π}], {θ, 0, π/2}]
4
105 π (25 κ1^2 + 19 κ1 κ2 + 25 κ2^2)
```

## The second Term

Next we compute

$$1/4 \int (H[\theta, \delta])^2 d\delta / d\epsilon^2 d\mu[\theta, \delta + \epsilon q] = \int d\delta^2 / d\epsilon^2 d\mu[\theta, \delta + \epsilon q]$$

To compute this, we consider the expansion from the “Variation of the measure” section in which we had seen

$$\sqrt{A} + \frac{B\epsilon}{2\sqrt{A}} + \frac{(-B^2 + 2AC)\epsilon^2}{8A^{3/2}} + O[\epsilon]^3$$

Taking two derivatives essentially gives the last term. However, we need to multiply by 2. So, the correct integrand is

$$\text{Integralfunktion}[\theta\_ , \phi\_ ] = 1/2 \text{Ableitung2}[\theta, \phi] / (\text{Sqrt}[\text{Ableitung0}[\theta, \phi]]) - 1/4 \text{Ableitung1}[\theta, \phi]^2 / (\text{Sqrt}[\text{Ableitung0}[\theta, \phi]]^3);$$

This function needs to be integrated over  $\theta$  and  $\phi$ . We do not need to include any measure, since this function already contains the measure

$$\text{Ergebnis2} = \text{Integrate}[\text{Integrate}[\text{Integralfunktion}[\theta, \phi], \{\phi, 0, 2\pi\}], \{\theta, 0, \pi/2\}] - \frac{4}{105} \pi (5 \kappa_1^2 - 6 \kappa_1 \kappa_2 + 5 \kappa_2^2)$$

## The third Term

Finally, compute the mixed term

$$2 * 1/4 \int d\delta / d\epsilon (H[\theta, \delta + \epsilon q])^2 d\delta / d\epsilon d\mu[\theta, \delta + \epsilon q]$$

The factor of two is included as it is generated by the product rule!

Going back to the expansion

$$\sqrt{A} + \frac{B\epsilon}{2\sqrt{A}} + \frac{(-B^2 + 2AC)\epsilon^2}{8A^{3/2}} + O[\epsilon]^3$$

we see that the derivative of the measure is given as

$$\text{varmass}[\theta\_ , \phi\_ ] = \text{FullSimplify}[B / (2 \text{Sqrt}[A]) /. \{A \rightarrow \text{Ableitung0}[\theta, \phi], B \rightarrow \text{Ableitung1}[\theta, \phi]\}];$$

The derivative of  $H^2$  is implemented as

$$\text{MixedIntFunc}[\theta\_ , \phi\_ ] = \text{FullSimplify}[D[H[\theta, \phi, \epsilon]^2, \epsilon] /. \epsilon \rightarrow 0];$$

Putting the two functions together and including the factor  $2/4$  we get

$$\text{Ergebnis3} = 2/4 \text{Integrate}[\text{Integrate}[\text{MixedIntFunc}[\theta, \phi] \text{varmass}[\theta, \phi], \{\phi, 0, 2\pi\}], \{\theta, 0, \pi/2\}] - \frac{16}{105} \pi (2 \kappa_1^2 - \kappa_1 \kappa_2 + 2 \kappa_2^2)$$

## Final Result

Combining all terms from above, we get

**Ergebnis = FullSimplify[Ergebnis1 + Ergebnis2 + Ergebnis3]**

$$\frac{4}{105} \pi (12 \kappa_1^2 + 29 \kappa_1 \kappa_2 + 12 \kappa_2^2)$$

We now replace  $\kappa_1$  and  $\kappa_2$  by their respective formulas in terms of H and K. This gives Equation (5.6)

**Expand[FullSimplify[  
 Ergebnis /. { $\kappa_1 \rightarrow \frac{1}{2} (H + \text{Sqrt}[H^2 - 4 K])$ ,  $\kappa_2 \rightarrow \frac{1}{2} (H - \text{Sqrt}[H^2 - 4 K])$ }]]]**

$$\frac{16 H^2 \pi}{35} + \frac{4 K \pi}{21}$$

# Proof of Equation (5.7)

Let  $\eta$  denote the interior unit normal

along  $\partial (S^2)_+$ . Combining Equations (B.84) and (B.85)

$$D_1 \mathcal{W}[\theta, \delta] u''(\theta) = \int_{\partial(S^2)_+} \partial_\eta u''(\theta) dS = \int_{\partial(S^2)_+} \frac{d^2}{d\epsilon^2} B_1[\epsilon u'(\theta), \delta + \epsilon q]$$

where  $q := g'(0)$  with  $g'(0)$  from Equation (5.1) and where  $B_1$  is the first component of the boundary operator in Equation (3.2). Since  $\omega^3$  is a constant, we work instead with

$$\beta[u, g] = -g^{ij} \tilde{\text{deg}}(\omega, \partial_i f) \partial_j f^3$$

## Preliminaries

We implement the graph function  $u := u'(\theta)$  from Equation (5.3) :

$$\omega_1[\theta, \phi] = \cos[\phi] \sin[\theta];$$

$$\omega_2[\theta, \phi] = \sin[\phi] \sin[\theta];$$

$$\omega_3[\theta, \phi] = \cos[\theta];$$

$$f[\theta, \phi] = (\kappa_1 \omega_1[\theta, \phi]^2 + \kappa_2 \omega_2[\theta, \phi]^2) \omega_3[\theta, \phi];$$

$$v_1[\theta, \phi] = 1 - \log[2] + 1/2 \log[1 + \omega_3[\theta, \phi]] - 3/4 \omega_3[\theta, \phi];$$

$$v_2[\theta, \phi] = (\omega_1[\theta, \phi]^2 - \omega_2[\theta, \phi]^2) / (1 + \omega_3[\theta, \phi]);$$

$$v[\theta, \phi] = (\kappa_1 + \kappa_2) v_1[\theta, \phi] + (\kappa_1 - \kappa_2) / 4 v_2[\theta, \phi];$$

$$u[\theta, \phi] = v[\theta, \phi] - 1/2 f[\theta, \phi];$$

as well as the metric from Equation (5.1)

$$q[x, y] = \{\{\theta, \theta, \kappa_1 x\}, \{\theta, \theta, \kappa_2 y\}, \{\kappa_1 x, \kappa_2 y, \theta\}\};$$

$$\tilde{\text{deg}}[x, y, \epsilon] = \text{IdentityMatrix}[3] + \epsilon q[x, y];$$

Additionally we put

$$e_1 = \{1, \theta, \theta\};$$

$$e_2 = \{\theta, 1, \theta\};$$

$$e_3 = \{\theta, \theta, 1\};$$

to be the standard basis in  $\mathbb{R}^3$ . Let

$$\psi_0[\theta, \phi] = \{\omega_1[\theta, \phi], \omega_2[\theta, \phi], \omega_3[\theta, \phi]\};$$

denote the spherical coordinate system. Our surface is given by

$$\psi u[\theta, \phi, \epsilon] = (1 + u[\theta, \phi] \epsilon) \psi_0[\theta, \phi];$$

On the surface, the metric is given by

$$\tilde{\text{degm}}[\theta, \phi, \epsilon] = \tilde{\text{deg}}[\psi u[\theta, \phi, \epsilon].e_1, \psi u[\theta, \phi, \epsilon].e_2, \epsilon];$$

## First Fundamental Form

The first fundamental form is given by

```
g11[θ_, ϕ_, ε_] = D[ψu[θ, ϕ, ε], θ].tildegm[θ, ϕ, ε].D[ψu[θ, ϕ, ε], θ];
g12[θ_, ϕ_, ε_] = D[ψu[θ, ϕ, ε], θ].tildegm[θ, ϕ, ε].D[ψu[θ, ϕ, ε], ϕ];
g22[θ_, ϕ_, ε_] = D[ψu[θ, ϕ, ε], ϕ].tildegm[θ, ϕ, ε].D[ψu[θ, ϕ, ε], ϕ];
```

We collect these entries into a matrix

```
g[θ_, ϕ_, ε_] = {{g11[θ, ϕ, ε], g12[θ, ϕ, ε]}, {g12[θ, ϕ, ε], g22[θ, ϕ, ε]}};
```

We also implement the inverse

```
ginv[θ_, ϕ_, ε_] = Inverse[g[θ, ϕ, ε]];
```

## Implementation of $\beta$

We define four auxiliary functions:

```
A1[θ_, ϕ_, ε_] = -ginv[θ, ϕ, ε][[1, 1]]
  (tildegm[θ, ϕ, ε].ψ0[θ, ϕ]).D[ψu[θ, ϕ, ε], θ] (D[ψu[θ, ϕ, ε].e3, θ]);
A2[θ_, ϕ_, ε_] = -ginv[θ, ϕ, ε][[1, 2]] (tildegm[θ, ϕ, ε].ψ0[θ, ϕ]).D[ψu[θ, ϕ, ε], θ]
  (D[ψu[θ, ϕ, ε].e3, ϕ]);
A3[θ_, ϕ_, ε_] = -ginv[θ, ϕ, ε][[2, 1]] (tildegm[θ, ϕ, ε].ψ0[θ, ϕ]).D[ψu[θ, ϕ, ε], ϕ]
  (D[ψu[θ, ϕ, ε].e3, θ]);
A4[θ_, ϕ_, ε_] = -ginv[θ, ϕ, ε][[2, 2]] (tildegm[θ, ϕ, ε].ψ0[θ, ϕ]).D[ψu[θ, ϕ, ε], ϕ]
  (D[ψu[θ, ϕ, ε].e3, ϕ]);
```

In view of Equation (3.2) we then have

$$\beta[\epsilon u'(0), \delta + \epsilon g'(0)] = A1 + A2 + A3 + A4$$

Hence we are interested in

$$\beta[\theta_-, \phi_-, \epsilon_-] = A1[\theta, \phi, \epsilon] + A2[\theta, \phi, \epsilon] + A3[\theta, \phi, \epsilon] + A4[\theta, \phi, \epsilon];$$

Considering Equations (B.84) and (B.85) we have to take two derivatives with respect to  $\epsilon$  at  $\epsilon=0$ :

$$Q[\theta_-, \phi_-] = D[\beta[\theta, \phi, \epsilon], \{\epsilon, 2\}] /. \epsilon \rightarrow 0;$$

Still considering Equations (B.84) and (B.85)

$$\text{Integral} := \int_{\partial(S^2)_+} \partial_\eta u''(\theta) dS = \int_{\partial(S^2)_+} Q dS$$

Since both integrals are boundary integrals over  $\partial S_+^2$ . So we only need  $\theta=\pi/2$ . So we implement

$$Q\text{Boundary}[\phi_-] = Q[\pi/2, \phi];$$

The boundary is parameterized as  $(\text{Cos}[\phi], \text{Sin}[\phi], 0)$ . This parameterization has first fundamental form (1). Hence, the line element along the boundary is one and so we need to compute

$$\text{Integral} = \text{Integrate}[Q\text{Boundary}[\phi], \{\phi, 0, 2\pi\}]$$

$$4\pi (\kappa_1 + \kappa_2)^2 (-1 + \text{Log}[2])$$

Since  $\kappa_1 + \kappa_2 = H$ , Equation (5.7) is established.
